# Supplementary material for: Density fitting in periodic systems: application to TDHF in diamond and oxides
Source: arXiv:2005.09291 source file (2020-05-19)
Supplement: Supplementary file 1 [file Supplementary_Information.pdf]

Supplementary Information for

# Density fitting in periodic systems: application to TDHF in diamond and oxides

by C. H. Patterson, School of Physics, Trinity College Dublin, Dublin 2, Ireland

This document contains details of wave function basis sets for C, O, Mg and Ti used in this work. DEF2-TZVP basis sets [1] and their corresponding DEF2-TZVP-RIFIT auxiliary basis sets were downloaded from www.basissetexchange.org [2] and modified for the solid state as indicated below. Basis functions whose exponents are in **bold** have been modified from those in the original basis set and those whose exponents are in **bold red** were omitted.

```
#BASIS SET: (11s,6p,2d,1f) -> [5s,3p,2d,1f]
C    S
  13575.3496820              0.22245814352E-03
   2035.2333680              0.17232738252E-02
    463.22562359             0.89255715314E-02
    131.20019598             0.35727984502E-01
     42.853015891            0.11076259931
     15.584185766            0.24295627626
C    S
      6.2067138508           0.41440263448
      2.5764896527           0.23744968655
C    S
      0.57696339419          1.0000000
C    S
      0.57700000000          1.0000000
C    S
      0.20000000000          1.0000000
C    P
     34.697232244            0.53333657805E-02
      7.9582622826           0.35864109092E-01
      2.3780826883           0.14215873329
      0.81433208183          0.34270471845
C    P
      0.50000000000          1.0000000
C    P
      0.20000000000          1.0000000
C    D
      1.09700000             1.0000000
C    D
      0.31800000             1.0000000
C    F
      0.76100000             1.0000000
```

```
#BASIS SET: (11s,6p,2d,1f) -> [5s,3p,2d,1f]
O    S
  27032.3826310              0.21726302465E-03
   4052.3871392              0.16838662199E-02
    922.32722710             0.87395616265E-02
    261.24070989             0.35239968808E-01
     85.354641351            0.11153519115
     31.035035245            0.25588953961
O    S
     12.260860728            0.39768730901
      4.9987076005           0.24627849430
O    S
      1.1703108158           1.0000000
O    S
      0.6474740994           1.0000000
O    S
      0.30000000000          1.0000000
O    P
     63.274954801            0.60685103418E-02
     14.627049379            0.41912575824E-01
      4.4501223456           0.16153841088
      1.5275799647           0.35706951311
O    P
      0.72935117943          0.44794207502
O    P
      0.300000000            1.0000000
O    D
      2.31400000             1.0000000
O    D
      0.50000000             1.0000000
O    F
      1.42800000             1.0000000
```

```
#BASIS SET: (14s,8p,3d) -> [5s,4p,3d]
Mg    S
  31438.3495550              0.60912311326E-03
   4715.5153354              0.47066196465E-02
   1073.1629247              0.24135820657E-01
    303.57238768             0.93628959834E-01
     98.626251042            0.26646742093
     34.943808417            0.47890929917
     12.859785199            0.33698490286
Mg    S
     64.876913004            0.19180889307E-01
     19.725520777            0.90913704392E-01
      2.8951804339          -0.39563756125
Mg    S
      1.1960454710           1.6827603373
      0.74329451156          0.52141091954
Mg    S
      0.30099104092          1.0000000
Mg    S
      0.36865728085E-01      1.0000000
Mg    P
    179.87189612             0.53799549018E-02
     42.120069376            0.39318014098E-01
     13.120503032            0.15740129476
      4.6257503609           0.35919094128
      1.6695211016           0.45533379310
Mg    P
      0.58551012105          0.21986432910
Mg    P
      0.30000000000          1.0000000
Mg    P
      0.53768755187E-01      1.0000000
Mg    D
      3.4440000              1.0000000
Mg    D
      0.5000000              1.0000000
Mg    D
      0.0700000              1.0000000
```

```
#BASIS SET: (17s,11p,7d,1f) -> [6s,4p,4d,1f]
Ti    S
 211575.6902500              0.23318151011E-03
  31714.9450580              0.18079690851E-02
   7217.5476543              0.93984311352E-02
   2042.9394247              0.38156853618E-01
    665.12896208             0.12374757197
    238.74942264             0.29208551143
     92.508691001            0.41226800855
     36.403919209            0.21090534061
Ti    S
    232.72624607            -0.24920140738E-01
     71.791209711           -0.11746490087
     11.158534615            0.56503342318
      4.6548135416           0.56211101812
Ti    S
      6.8034629174          -0.23011425503
      1.1201076403           0.72103186735
Ti    S
      0.48080118839          1.0000000
Ti    S
      0.85157274977E-01      1.0000000
Ti    S
      0.32657477046E-01      1.0000000
Ti    P
   1063.1474732              0.24690839320E-02
    251.56507061             0.19773345523E-01
     80.408554854            0.90987976672E-01
     29.768193269            0.25559900413
     11.736830556            0.40489386764
      4.7142375230           0.23693402558
Ti    P
     17.796803704           -0.27878639615E-01
      2.4272698680           0.55672914668
      0.96823445537          1.0055447350
Ti    P
      0.37056694165          1.0000000
Ti    P
      0.1015610              1.0000000
Ti    D
     37.713384723            0.11513835092E-01
     10.692931184            0.67246343996E-01
      3.6728446990           0.21484207775
      1.3588590303           0.38890892779
Ti    D
      0.49213295253          1.0000000
Ti    D
      0.16330520653          1.0000000
Ti    D
      0.0540000              1.0000000
Ti    F
      0.5620000              1.0000000
```


[1] F. Weigend and R. Ahlrichs, Balanced basis sets of split valence, triple zeta valence and quadruple zeta valence quality for H to Rn: Design and assessment of accuracy, Phys. Chem. Chem. Phys.7, 3297 (2005).

[2] B. P. Pritchard, D. Altarawy, B. Didier, T. D. Gibsom and T. L. Windus, *A New Basis Set Exchange: An Open, Up-to-date Resource for the Molecular Sciences Community.*J. Chem. Inf. Model. **59**, 4814 (2019).
